# Supplementary material for: Calendar Graph Neural Networks for Modeling Time Structures in Spatiotemporal User Behaviors
Source: arXiv:2006.06820 source file (2020-07-17)
Supplement: Supplementary file 1 [file 7appendix.tex]

\section{Reproducibility Justification}
This section provides a justification of the proposed method's reproducibility, covering information necessary for reproducing the experimental results, insights, or conclusions reported in the paper.
We first list out online resources including (i) a reference implementation of \textsc{CalendarGNN}; and, (ii) 2 real spatiotemporal behavior datasets used in Section~\ref{sec:experiments}. Then, we provide more details on parameter settings of \textsc{CalendarGNN} and all baseline methods.

\subsection{Code Package}

Our open-source code package is available on Github:
\begin{quote}
    \url{https://github.com/kdd2020calendargnn/CalendarGNN}
\end{quote}

\subsection{Datasets}
The 2 real spatiotemporal behavior logs $\mathcal{B}^{(w1)}$ and $\mathcal{B}^{(w2)}$ of users (after anonymization) are available at:
\begin{itemize}
	\item \makebox[0.45in][l]{$\mathcal{B}^{(w1)}$}: \url{https://bit.ly/2SpocOD}
	\item \makebox[0.45in][l]{$\mathcal{B}^{(w2)}$}: \url{https://bit.ly/2SM1T4T}
\end{itemize}

\subsection{Parameter Settings}
Our \textsc{CalendarGNN} (and \textsc{CalendarGNN-Attn}) was implemented in \text{PyTorch} \cite{paszke2017automatic}. We use {Stochastic Gradient Descent} \cite{bottou2010large} and {AMDM} \cite{kingma2014adam} updating rule with initial learning rate $\alpha=10^{-4}$ for training.
We set the dimensions as 256 for session embeddings (i.e., $K_\mathcal{S}$) and all spatial/temporal unit embeddings, (i.e., $K_h$, $K_w$, $K_y$, and $K_l$). And, the dimensions for all spatial/temporal patterns (i.e., $K_{\mathcal{T}_h}$, $K_{\mathcal{T}_w}$, $K_{\mathcal{T}_y}$, and $K_{\mathcal{L}}$) are set as 128. The dimensions of user final representation $K_{\mathcal{U}}$ is $512=128\times 4$ for \textsc{CalendarGNN}, and equals $768=(128+128)\times 3$ for \textsc{CalendarGNN-Attn}. Besides, due to anonymization, the features for items nodes $\mathcal{V}$ and locations nodes $\mathcal{L}$ provided in the above open datasets only include the identification information.

We use open-source code packages provided by the original paper for all baseline methods and follow the setup guidelines provided by the authors when possible.
For \textsc{ECC}, we pass in session/item/location as different labels for graph nodes and pass in session-item, or session-location, as different labels for graph edges.
For \textsc{DiffPool}, we use \textsc{GraphSAGE} \cite{hamilton2017inductive} as the base model, augment the training process with auxiliary link prediction signal plus entropy regularization, and set the number of clusters as $25\%$ of input nodes.
For \textsc{DCGNN}, the $k$ of the \textsc{SortPooling} layer is set that $90\%$ of graphs have nodes more than $k$.
For \textsc{CapsGNN}, we set the number of node/graph capsules as 2 and the dimension of graph/class capsules as 4.
For \textsc{SAGPool}, we use the hierarchical/serial architecture with pooling ratio set to $25\%$.
For \textsc{LearnSuc}, we set uniform weights for all item types and use the type-distribution-constrained negative sampling strategy with size of 10.
We directly use the session embeddings of user generated by \textsc{SR-GNN} for downstream tasks.
The \textit{scikit-learn} implementation % \cite{scikit-learn}
is used for \textsc{LR} models.

To make fair comparisons, we consistently set the dimensions of final user embeddings the same across models, and set the penultimate layer, i.e., the prediction model, as a fully connected layer for all methods. Also, the same $80\%/10\%/10\%$ split of training, validation and test users are shared by all methods for each run.
All neural models are trained for a maximum of 100 epochs with early stopping criteria applied when the validation loss keeps non-decreasing for 3 consecutive epochs. Saved model with best performance on the validation set is used for prediction on the test user set. We report the average performance metrics of 5 runs starting with different random seeds.

\begin{table*}[t]
	
	\centering
	\caption{For dataset $\mathcal{B}^{(w1)}$, the performance of CalendarGNN's ablated variants on classifying/predicting user labels (i) binary gender $\mathcal{A}^{(gen)}$, (ii) 10-classes income level $\mathcal{A}^{(inc)}$, and (iii) numerical age $\mathcal{A}^{(age)}$.} % For all metrics except error-based MAE and RMSE, higher values indicate better model performance.}
	\label{tab:results_ablation_nyr}
	\vspace{-0.15in}
	\Scale[0.92]{
	\begin{tabular}{|l||c|c|c|c|c|c|c|c|c|c|c|c|}
	\hline
		\multirow{2}*{\textbf{Method}} & \multicolumn{4}{|c|}{\textbf{Gender} $\mathcal{A}^{(gen)}$} & \multicolumn{4}{|c|}{\textbf{Income} $\mathcal{A}^{(inc)}$} & \multicolumn{4}{|c|}{\textbf{Age} $\mathcal{A}^{(age)}$} \\ \cline{2-13}
		 & {$Acc.$} & {$AUC$} & {$F1$} & {$MCC$} & {$Acc.$} & {$F1$-macro} & {$F1$-micro} & {Cohen's kappa $\kappa$} & {$R^{2}$} & {$MAE$} & {$RMSE$} & {Pearson's $r$}  \\ \hline \hline
		\textsc{CalendarGNN}($\mathbf{s}$)		& {70.59\%} & {.6721} & {.6812} & {.4063} & {24.89\%} & {.0622} & {.2603} & {.0280} & {.2154} & {11.59} & {14.97} & {.4702}  \\ \hline
		\textsc{CalendarGNN}($-\mathbf{p}_{\mathcal{T}_h}$) 	& {71.12\%} & {.6770} & {.6892} & {.4139} & {25.09\%} & {.0738} & {.2650} & {.0354} & {.2199} & {11.32} & {14.56} & {.4722}  \\ \hline
		\textsc{CalendarGNN}($-\mathbf{p}_{\mathcal{T}_w}$) 	& {71.97\%} & {.6993} & {.7032} & {.4387} & {26.45\%} & {.0830} & {.2802} & {.0742} & {.2319} & {11.09} & {14.20} & {.4830}  \\ \hline
		\textsc{CalendarGNN}($-\mathbf{p}_{\mathcal{T}_y}$) 	& {72.07\%} & {.7181} & {.7072} & {.4423} & {27.67\%} & {.0882} & {.2890} & {.0809} & {.2185} & {11.38} & {14.80} & {.4630}  \\ \hline
		\textsc{CalendarGNN}($-\mathbf{p}_{\mathcal{L}}$) 	& {72.63\%} & {.7239} & {.7104} & {.4484} & {25.04\%} & {.0676} & {.2680} & {.0421} & {.2380} & {10.96} & {13.96} & {.4930}  \\ \hline
		\hline
		\textsc{CalendarGNN} 		& {72.98\%} & {.7250} & {.7119} & {.4503} & {28.83\%} & {.1059} & {.2981} & {.0887} & {.2412} & {10.57} & {13.60} & {.5033}  \\ \hline
	\end{tabular}
	}
\end{table*}

\begin{table*}[t]
	
	\centering
	\caption{For dataset $\mathcal{B}^{(w2)}$, the performance of CalendarGNN's ablated variants on classifying/predicting user labels (i) binary gender $\mathcal{A}^{(gen)}$, (ii) 10-classes income level $\mathcal{A}^{(inc)}$, and (iii) numerical age $\mathcal{A}^{(age)}$.} % For all metrics except error-based MAE and RMSE, higher values indicate better model performance.}
	\label{tab:results_ablation_vnf}
	\vspace{-0.15in}
	\Scale[0.92]{
	\begin{tabular}{|l||c|c|c|c|c|c|c|c|c|c|c|c|}
	\hline
		\multirow{2}*{\textbf{Method}} & \multicolumn{4}{|c|}{\textbf{Gender} $\mathcal{A}^{(gen)}$} & \multicolumn{4}{|c|}{\textbf{Income} $\mathcal{A}^{(inc)}$} & \multicolumn{4}{|c|}{\textbf{Age} $\mathcal{A}^{(age)}$} \\ \cline{2-13}
		 & {$Acc.$} & {$AUC$} & {$F1$} & {$MCC$} & {$Acc.$} & {$F1$-macro} & {$F1$-micro} & {Cohen's kappa $\kappa$} & {$R^{2}$} & {$MAE$} & {$RMSE$} & {Pearson's $r$}  \\ \hline \hline
		\textsc{CalendarGNN}($\mathbf{s}$)		& {69.23\%} & {.6610} & {.6729} & {.3829} & {23.58\%} & {.0598} & {.2434} & {.0216} & {.1952} & {12.14} & {15.39} & {.4429}  \\ \hline
		\textsc{CalendarGNN}($-\mathbf{p}_{\mathcal{T}_h}$) 	& {69.89\%} & {.6723} & {.6790} & {.3892} & {24.21\%} & {.0628} & {.2458} & {.0386} & {.2010} & {11.79} & {14.75} & {.4506}  \\ \hline
		\textsc{CalendarGNN}($-\mathbf{p}_{\mathcal{T}_w}$) 	& {70.48\%} & {.6921} & {.6876} & {.4120} & {26.72\%} & {.0882} & {.2704} & {.0698} & {.2120} & {11.40} & {14.20} & {4632}  \\ \hline
		\textsc{CalendarGNN}($-\mathbf{p}_{\mathcal{T}_y}$) 	& {70.80\%} & {.6984} & {.6906} & {.4272} & {26.67\%} & {.0874} & {.2698} & {.0700} & {.2032} & {12.40} & {15.59} & {.4489}  \\ \hline
		\textsc{CalendarGNN}($-\mathbf{p}_{\mathcal{L}}$) 	& {71.12\%} & {.7020} & {.6949} & {.4309} & {24.03\%} & {.0625} & {.2459} & {.0324} & {.2163} & {10.97} & {14.02} & {.4803}  \\ \hline
		\hline
		\textsc{CalendarGNN} 		& {71.63\%} & {.7104} & {.7038} & {.4389} & {27.10\%} & {.0909} & {.2798} & {.0742} & {.2223} & {10.79} & {13.88} & {.4872}  \\ \hline
	\end{tabular}
	}
\end{table*}

\section{Additional Experimental Results}
This section provides more experimental results not fully covered in Section \ref{sec:experiments} for validating the effectiveness of the proposed method.
\subsection{Ablation Test}
To validate to importantce of each spatiotemporal pattern ($\mathbf{p}_{\mathcal{T}_h}$, $\mathbf{p}_{\mathcal{T}_w}$, $\mathbf{p}_{\mathcal{T}_y}$, a nd $\mathbf{p}_{\mathcal{L}}$) for predicting different user labels, we further devise 5 variants of \textsc{CalendarGNN} by removing each single pattern from the final user embedding and examine their performances. These 5 ablated versions of \textsc{CalendarGNN} include:
\begin{compactitem}
	\item \textsc{CalendarGNN}($\mathbf{s}$): No spatial or temporal pattern is generated. A \textsc{GRU} layer is applied on session embeddings $\{\mathbf{s}~|~s \in S\}$ and the last hidden state is used for prediction,
	\item \textsc{CalendarGNN}($-\mathbf{p}_{\mathcal{T}_h}$): The hourly pattern $\mathbf{p}_{\mathcal{T}_h}$ is removed from the final user embedding $\mathbf{u}$,
	\item \textsc{CalendarGNN}($-\mathbf{p}_{\mathcal{T}_w}$): The weekly pattern $\mathbf{p}_{\mathcal{T}_w}$ is removed from the final user embedding $\mathbf{u}$,
	\item \textsc{CalendarGNN}($-\mathbf{p}_{\mathcal{T}_y}$): The weekday pattern $\mathbf{p}_{\mathcal{T}_y}$ is removed from the final user embedding $\mathbf{u}$,
	\item \textsc{CalendarGNN}($-\mathbf{p}_{\mathcal{L}}$): The spatial pattern $\mathbf{p}_{\mathcal{L}}$ is removed from the final user embedding $\mathbf{u}$.
\end{compactitem}
The results of these \textsc{CalendarGNN}'s variants on predicting user labels on two dataset are provided in Table \ref{tab:results_ablation_nyr} and \ref{tab:results_ablation_vnf}, respectively.

\subsubsection{Hourly pattern}
The hourly pattern $\mathbf{p}_{\mathcal{T}_h}$ makes most of the contributions to the effectiveness of \textsc{CalendarGNN} among all four patterns.
Without the hourly pattern $\mathbf{p}_{\mathcal{T}_h}$, \textsc{CalendarGNN}($-\mathbf{p}_{\mathcal{T}_h}$) scores an Acc. of $71.12\%$ for predicting user gender $\mathcal{A}^{(gen)}$, an Acc. of $25.09\%$ for predicting user income $\mathcal{A}^{(inc)}$, and an RMSE of $14.56$ for predicting user age $\mathcal{A}^{(age)}$ on dataset $\mathcal{B}^{(w1)}$. After incorporating $\mathbf{p}_{\mathcal{T}_h}$ in the user embedding $\mathbf{u}$, \textsc{CalendarGNN} is able to improve upon \textsc{CalendarGNN}($-\mathbf{p}_{\mathcal{T}_h}$) by $+2.62\%$, $+14.91\%$, and $-6.59\%$ for Acc. of predicting $\mathcal{A}^{(gen)}$, Acc. of predicting $\mathcal{A}^{(inc)}$, and RMSE of predicting $\mathcal{A}^{(age)}$ respectively.
Similarly, on dataset $\mathcal{B}^{(w2)}$, without the hourly pattern $\mathbf{p}_{\mathcal{T}_h}$, \textsc{CalendarGNN}($-\mathbf{p}_{\mathcal{T}_h}$) scores an Acc. of $69.89\%$ for predicting user gender $\mathcal{A}^{(gen)}$, an Acc. of $24.21\%$ for predicting user income $\mathcal{A}^{(inc)}$, and an RMSE of $14.75$ for predicting user age $\mathcal{A}^{(age)}$. After incorporating $\mathbf{p}_{\mathcal{T}_h}$ in the user embedding $\mathbf{u}$, \textsc{CalendarGNN} is able to improve upon \textsc{CalendarGNN}($-\mathbf{p}_{\mathcal{T}_h}$) by $+2.49\%$, $+11.94\%$, and $-5.90\%$ for Acc. of predicting $\mathcal{A}^{(gen)}$, Acc. of predicting $\mathcal{A}^{(inc)}$, and RMSE of predicting $\mathcal{A}^{(age)}$ respectively.
This indicates that user's temporal pattern of hourly periodicity is critical for predicting user demographic labels. 

\subsubsection{Weekly pattern}
The weekly pattern $\mathbf{p}_{\mathcal{T}_w}$ makes lots of contributions to the effectiveness of \textsc{CalendarGNN} but not as much as the hourly pattern $\mathbf{p}_{\mathcal{T}_h}$. 
On dataset $\mathcal{B}^{(w1)}$, without the weekly pattern $\mathbf{p}_{\mathcal{T}_w}$, \textsc{CalendarGNN}($-\mathbf{p}_{\mathcal{T}_w}$) scores an Acc. of $71.97\%$ for predicting user gender $\mathcal{A}^{(gen)}$, an Acc. of $26.45\%$ for predicting user income $\mathcal{A}^{(inc)}$, and an RMSE of $14.20$ for predicting user age $\mathcal{A}^{(age)}$. After incorporating $\mathbf{p}_{\mathcal{T}_w}$ in the user embedding $\mathbf{u}$, \textsc{CalendarGNN} is able to improve upon \textsc{CalendarGNN}($-\mathbf{p}_{\mathcal{T}_w}$) by $+1.40\%$, $+9.00\%$, and $-4.23\%$ for Acc. of predicting $\mathcal{A}^{(gen)}$, Acc. of predicting $\mathcal{A}^{(inc)}$, and RMSE of predicting $\mathcal{A}^{(age)}$ respectively. The improvements brought by incorporating $\mathbf{p}_{\mathcal{T}_w}$ in the user embedding $\mathbf{u}$ is slightly lower than incorporating $\mathbf{p}_{\mathcal{T}_h}$. The similar trend can also be observed on the dataset $\mathcal{B}^{(w2)}$.

\subsubsection{Weekday pattern}
The weekday pattern $\mathbf{p}_{\mathcal{T}_y}$ makes significant contributions to the effectiveness of \textsc{CalendarGNN} for predicting user age $\mathcal{A}^{(age)}$ across two datasets. On dataset $\mathcal{B}^{(w1)}$, without the weekday pattern $\mathbf{p}_{\mathcal{T}_y}$, \textsc{CalendarGNN}($-\mathbf{p}_{\mathcal{T}_y}$) scores an RMSE of $14.80$ for predicting user age $\mathcal{A}^{(age)}$. After incorporating $\mathbf{p}_{\mathcal{T}_y}$ in the user embedding $\mathbf{u}$, \textsc{CalendarGNN} is able to improve upon \textsc{CalendarGNN}($-\mathbf{p}_{\mathcal{T}_y}$) by $-8.11\%$. 
This observation is also consistent on dataset $\mathcal{B}^{(w2)}$.
%On dataset $\mathcal{B}^{(w2)}$, without the weekday pattern $\mathbf{p}_{\mathcal{T}_y}$, \textsc{CalendarGNN}($-\mathbf{p}_y$) scores an RMSE of $15.59$ for predicting user age $\mathcal{A}^{(age)}$. After incorporating $\mathbf{p}_{\mathcal{T}_y}$ in the user embedding $\mathbf{u}$, \textsc{CalendarGNN} is able to improve upon \textsc{CalendarGNN}($-\mathbf{p}_{\mathcal{T}_y}$) by $-10.97\%$.
And, this tells that the weekday pattern $\mathbf{p}_y$ is especially useful for predicting user age information.

\subsubsection{Spatial pattern}
The spatial pattern $\mathbf{p}_{\mathcal{L}}$ plays an important role for predicting user income $\mathcal{A}^{(inc)}$. This follows our intuition that the location signal of the user might be indicative about his income level. For example, users with location item of ``\textit{US/New York/New York}'' might have higher income than users from small townships. 
On dataset $\mathcal{B}^{(w1)}$, without the spatial pattern $\mathbf{p}_{\mathcal{L}}$, \textsc{CalendarGNN}($-\mathbf{p}_{\mathcal{L}}$) scores an Acc. of $28.83\%$ for predicting user income $\mathcal{A}^{(inc)}$. After incorporating $\mathbf{p}_{\mathcal{L}}$ in the user embedding $\mathbf{u}$, \textsc{CalendarGNN} is able to improve upon \textsc{CalendarGNN}($-\mathbf{p}_{\mathcal{L}}$) by $+15.14\%$.
The similar trend can also be observed on dataset $\mathcal{B}^{(w2)}$.
%On dataset $\mathcal{B}^{(w2)}$, without the spatial pattern $\mathbf{p}_{\mathcal{L}}$, \textsc{CalendarGNN}($-\mathbf{p}_{\mathcal{L}}$) scores an Acc. of $27.10\%$ for predicting user income $\mathcal{A}^{(inc)}$. After incorporating $\mathbf{p}_{\mathcal{L}}$ in the user embedding $\mathbf{u}$, \textsc{CalendarGNN} is able to improve upon \textsc{CalendarGNN}($-\mathbf{p}_{\mathcal{L}}$) by $+12.78\%$.

Since different patterns contribute differently to \textsc{CalendarGNN}'s predictive power on user label. We employ the attention mechanism introduced in Section \ref{sec:interactive} for dynamically adapting the importance of patterns and modeling their interactions. Besides, the proposed framework is also flexible for incorporating more patterns of different periodicity providing the time unit mapping function.
